# Supplementary material for: Absence of a transport signature of spin-orbit coupling in graphene with indium adatoms
Source: arXiv:1409.8090 ancillary file (2014-09-29)
Supplement: Supplementary file 1 [file SOC.in.G.supplementary.pdf]

# Supplemental material for: Absence of a Transport Signature of Spin-orbit Coupling in Graphene with Indium Adatoms

Zhenzhao Jia, Baoming Yan, Jingjing Niu, Qi Han, Rui Zhu, Xiaosong Wu,* and Dapeng Yu

*State Key Laboratory for Artificial Microstructure and Mesoscopic Physics,*

*Peking University, Beijing 100871, China*

*Collaborative Innovation Center of Quantum Matter, Beijing 100871, China*

Magnesium is a light element. It introduces little spin-orbit coupling (SOC)[1]. If indium can significantly enhances the SOC, the magnetotransport should be qualitatively different from magnesium. We have carried out the same experiment with Mg. The sample preparation processes are the same. Deposition of Mg was performed *in situ* at a very slow rate at a temperature below 5 K. During deposition, the resistance of the device was monitored so as to obtain a desired gate voltage shift of the Dirac point. After each deposition, transport measurements were performed at different gate voltages.

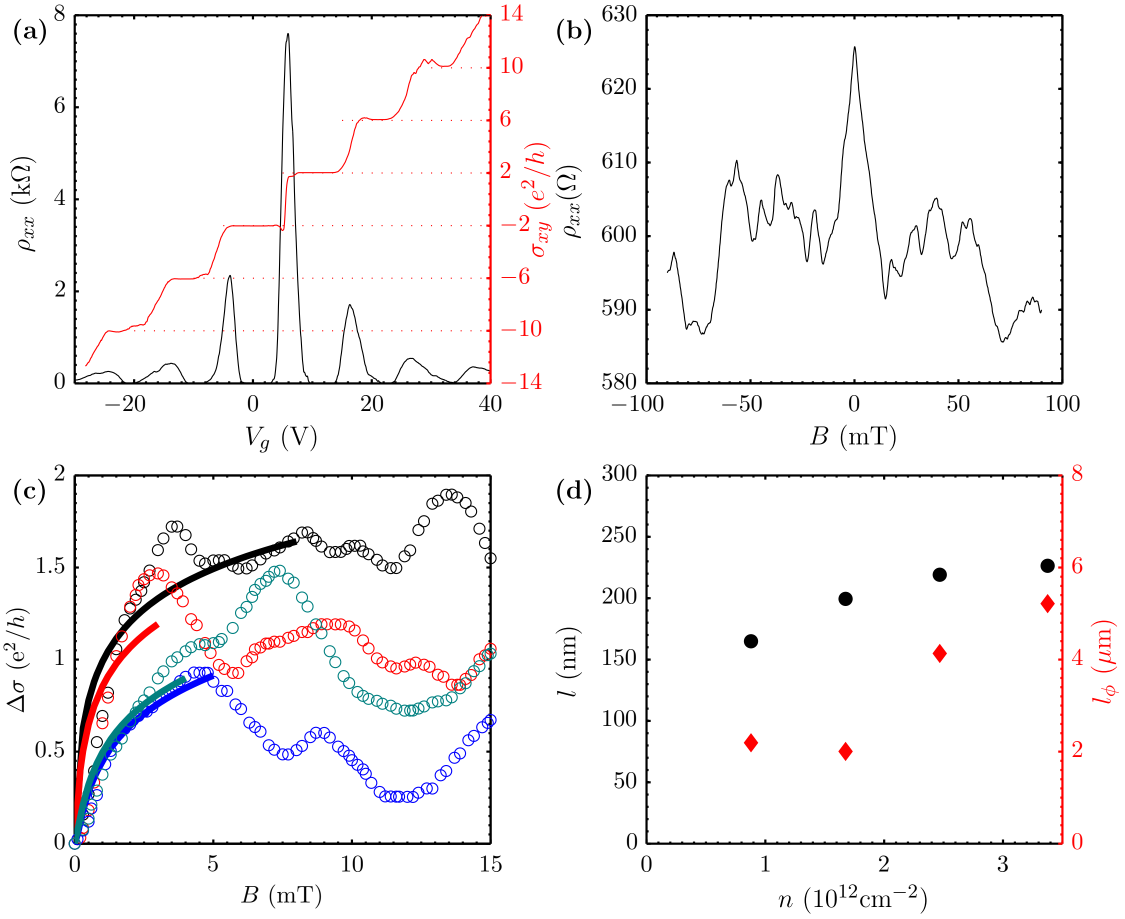


FIG. S1 Magnetotransport of a graphene Hall bar device before Mg deposition. (a) Longitudinal resistivity and the transverse conductivity versus the gate voltage in 9 T at 150 mK, showing the half integer quantum Hall effect. (b) Low field magnetoresistivity exhibits two features, the weak localization peak at $B = 0$ and the universal conductance fluctuations. (c) Fits to Eq. 1 in the main text for the low field magnetoresistivity at different carrier densities. (d) The mean free path $l$ and the phase coherence length $l_\phi$ as a function of $n_s$. $l_\phi$ is obtained from the fits in (c).

Magnetoresistance of pristine graphene before Mg deposition is shown in Fig. S1. The field effect mobility is 11400 $cm^2/Vs$. The sample exhibits the half integer quantum Hall effect, confirming that it is a monolayer. The low field resistance displays a weak localization peak around $B = 0$ and universal conductance fluctuations. By fitting the weak localization peak to Eq. 1 in the main text, the carrier density dependence of the phase coherence length $l_\phi$ is obtained and plotted in Fig. S1(d), as well as the mean free path $l$.

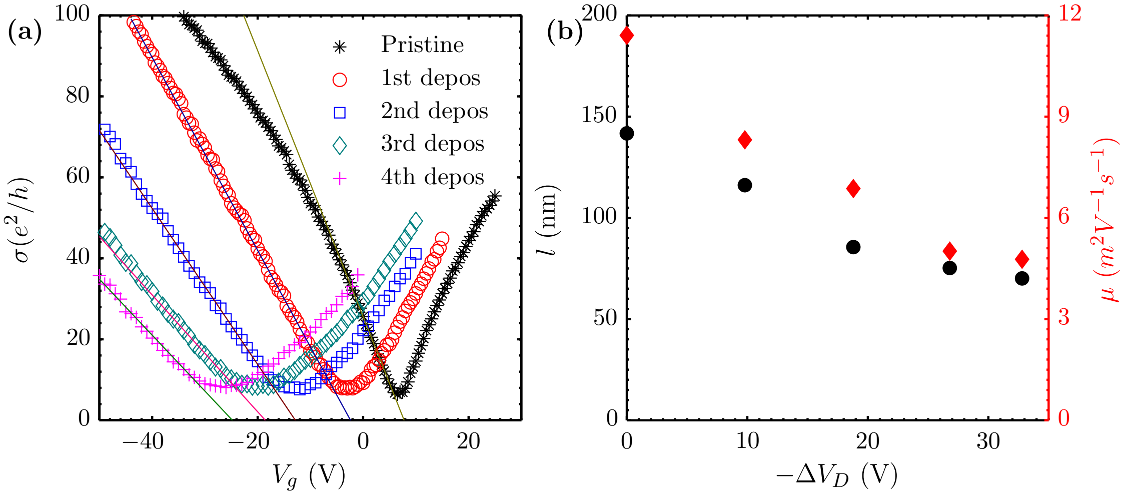


FIG. S2 Deposition of magnesium. (a) The conductivity $\sigma$ versus gate voltage $V_g$ curves for the device after each deposition. The solid lines are linear fits, from which the field effect mobility is obtained. (b) The dependence of the mean free time $\tau$ at a carrier density of $1.7 \times 10^{12}$ $cm^2/Vs$ and the field effect mobility $\mu$ on the shift of the Dirac point $\Delta V_D$.

In Fig. S2, the density dependence of the conductivity $\sigma$ for pristine graphene displays a sublinear behaviour at high density, suggesting noticeable short range scatterers[2]. Upon Mg deposition, the Dirac point shifts towards negative gate voltage due to electron doping. At the same time, the density dependence of $\sigma$ turns linear, indicating dominance of long range scatterers. This observation is consistent with In deposition. As these metal adatoms electron-dope graphene by charge transfer, they are positive charged. Scattering by these ionized adatoms is dictated by the long range Coulomb potential, instead of the short range component. This is in accordance with previous studies in which noticeable short range scattering occurs for insulating neutral absorbates[3, 4].

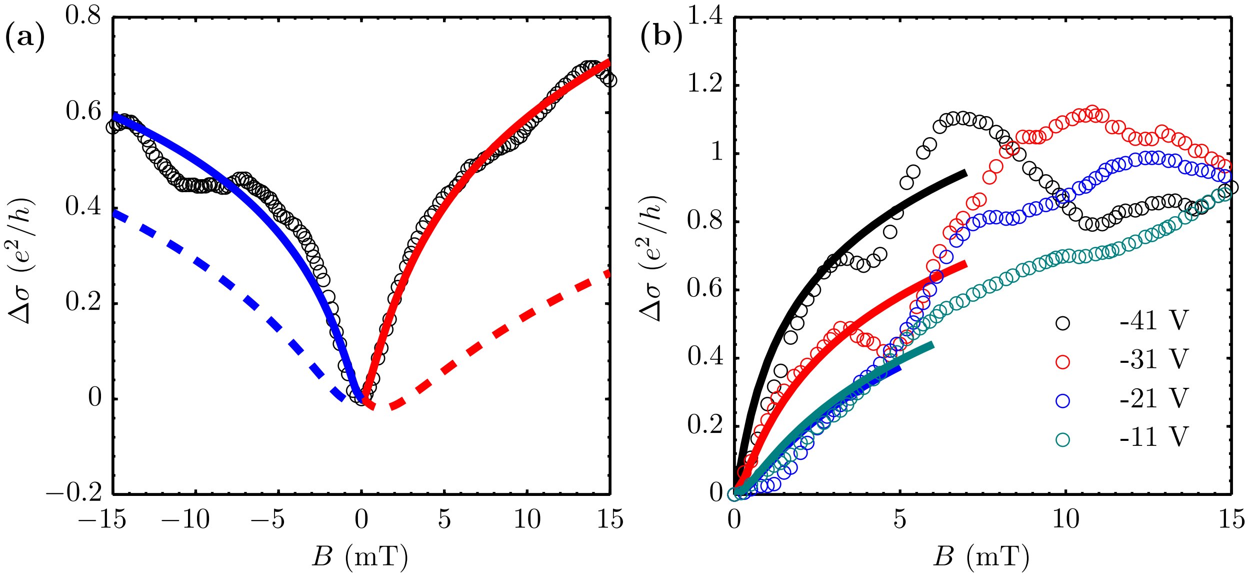


FIG. S3 Low field magnetoconductivity after the fourth deposition of Mg. (a) Fit of the low field magnetoconductivity at a carrier density of $1.7 \times 10^{12}$ cm$^2$/Vs to Eq. 1 and Eq. 2 in the main text. The circles are experimental data. The solid lines are the best fits to the equations, red for Eq. 1 and blue for Eq. 2. The dotted lines are the plot of two equations, assuming a spin-orbit scattering time $\tau_{\rm so} = \tau_\phi$. (b) Magnetoconductivity data and fits to Eq. 1 at different gate voltages relative to the Dirac point. The fluctuations of the conductivity are reproducible and due to universal conductance fluctuations.

The low field magnetoconductivity after deposition is shown in Fig. S3(a). It remains positive, as expected for negligible SOC. Eq. 1 and Eq. 2 are used to fit the data. The fit to Eq. 1 yields $\tau_\phi = 18.5$ ps, while the fit to Eq. 2 gives a similar value $\tau_\phi = 20.6$ ps. In both cases, the fitted $\tau_{\rm so}$ is much larger than $\tau_\phi$. The expected non-monotonic magnetoconductivity with increasing field for $\tau_{\rm so} = \tau_\phi$ is plotted in Fig. S3(a), in contrast to the monotonic behaviour of the experimental curve. Independent of any theory, the qualitatively same behaviour for In and Mg deposition confirms that no appreciable SOC is induced by In.

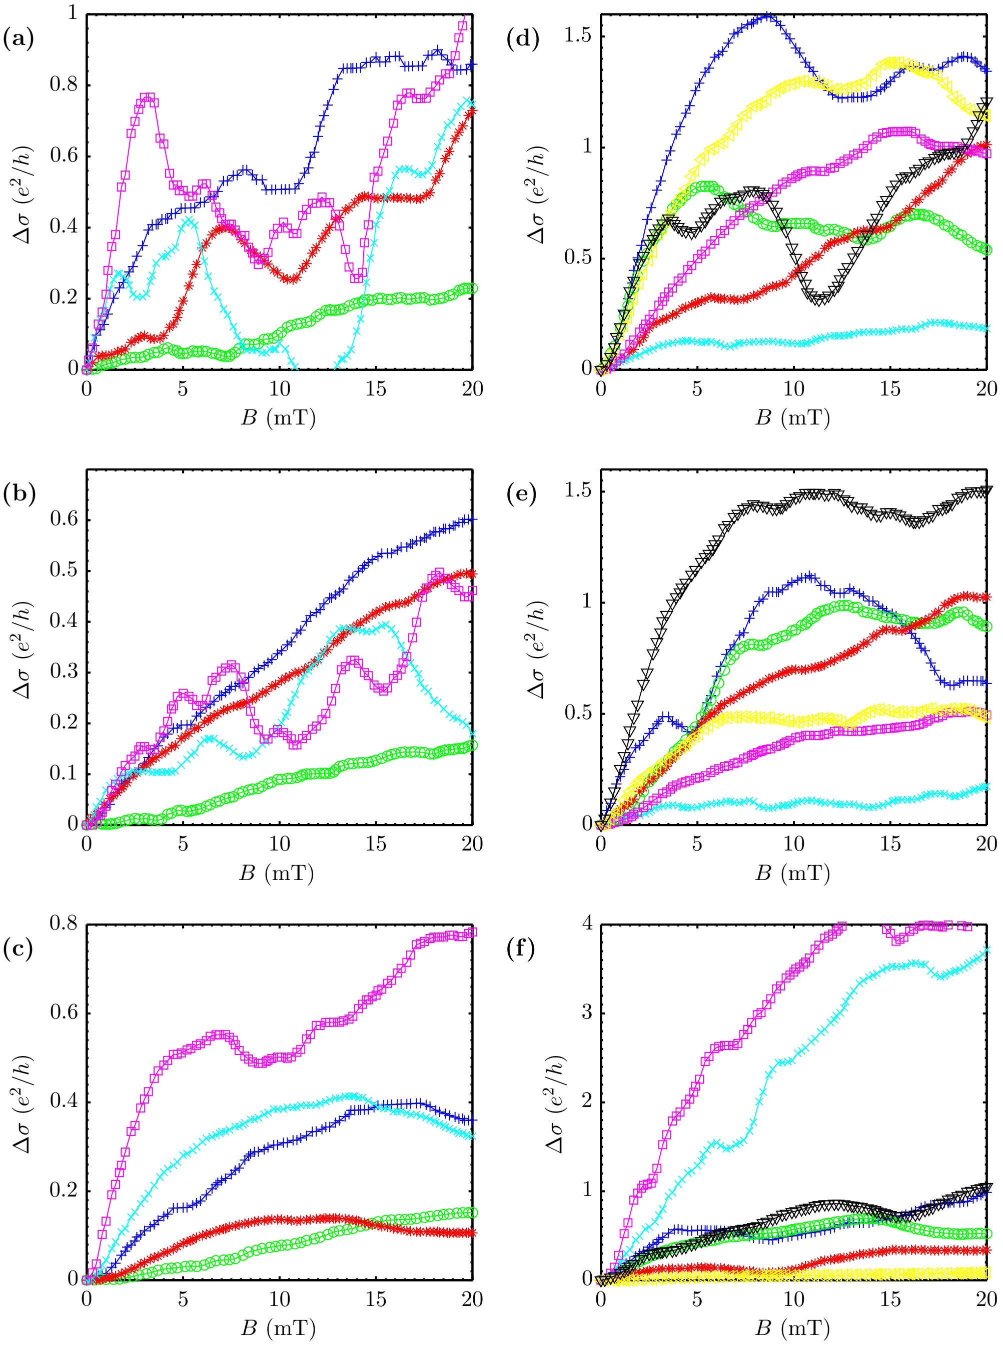


FIG. S4 Weak localization measurements at different carrier densities after the each deposition. (a)(d) After the first deposition.(b)(e) After the second deposition.(c)(f) After the third deposition. (a)-(c) Indium depositions. Different colors and markers stand for different gate voltages with respect to the Dirac point. +: -23 V, ○: -3 V, *: 17 V, ×: 37 V, □: 57 V. (d)-(f) Magnesium depositions. The gate voltage for +: -31 V, ○: -21 V, *: -11 V, ×: -1 V, □: 9 V, ◁: 19 V, ▽: is 29 V

After each deposition, we have scrutinized the low field magnetoconductivity at various carrier densities for evidence of weak antilocalization. Fig. S4 shows some of these curves. For comparison, we also plot the data for Mg deposition. Weak localization is evident. Not a single one displays a non-monotonic dependence near zero field.

* xswu@pku.edu.cn

[1] A. G. Swartz, J.-R. Chen, K. M. McCreary, P. M. Odenthal, W. Han, and R. K. Kawakami, Phys. Rev. B **87**, 075455 (2013).

[2] S. Adam, E. H. Hwang, V. M. Galitski, and S. Das Sarma, Proc. Natl. Acad. Sci. USA **104**, 18392 (2007).

[3] W. Zhu, D. Neumayer, V. Perebeinos, and P. Avouris, Nano Lett. **10**, 3572 (2010).

[4] K. M. McCreary, K. Pi, and R. K. Kawakami, Appl. Phys. Lett. **98**, 192101 (2011).
